# Supplementary material for: PANDORA: Polarization-Aided Neural Decomposition Of Radiance
Source: arXiv:2203.13458 source file (2022-03-25)
Supplement: Supplementary file 1 [file suppl_pol_vs_nopol.tex]

\begin{figure}[ht!]
\centering
\setlength{\tabcolsep}{0pt}
% \begin{tabular}{rcccc@{\hskip 3pt}|@{\hskip 3pt}cccc}
\begin{tabular}{rcccc@{\hskip 3pt}@{\hskip 3pt}cccc}
& Mixed & Diffuse & Specular & Surface
% & Mixed & Diffuse & Specular & Surface
\\
& Radiance & Radiance & Radiance & Normals
% & Radiance & Radiance & Radiance & Normals
\\

%%%%%%%%%%%%%%%%%%%%%%%%%%%%%%%
\rotatebox[origin=c]{90}{Unpolarized}&
\raisebox{-0.5\height}{\igr{0.12}{0.cm}{0.cm}{0.cm}{0.cm}
{out_imgs/sim_comparisons/globe_unpol/pred_000_cues_mix_s0.png}}&
\raisebox{-0.5\height}{\igr{0.12}{0.cm}{0.cm}{0.cm}{0.cm}
{out_imgs/sim_comparisons/globe_unpol/pred_000_rgb.png}}&
\raisebox{-0.5\height}{\igr{0.12}{0.cm}{0.cm}{0.cm}{0.cm}
{out_imgs/sim_comparisons/globe_unpol/pred_000_spec.png}}&
\raisebox{-0.5\height}{\igr{0.12}{0.cm}{0.cm}{0.cm}{0.cm}
{out_imgs/sim_comparisons/globe_unpol/pred_000_normal.png}}&
\\
%%%%%%%%%%%%%%%%%%%%%%%%%%%%%%%
\rotatebox[origin=c]{90}{Ours}&
\raisebox{-0.5\height}{\igr{0.12}{0.cm}{0.cm}{0.cm}{0.cm}
{out_imgs/sim_comparisons/globe_ours/pred_000_cues_mix_s0.png}}&
\raisebox{-0.5\height}{\igr{0.12}{0.cm}{0.cm}{0.cm}{0.cm}
{out_imgs/sim_comparisons/globe_ours/pred_000_rgb.png}}&
\raisebox{-0.5\height}{\igr{0.12}{0.cm}{0.cm}{0.cm}{0.cm}
{out_imgs/sim_comparisons/globe_ours/pred_000_spec.png}}&
\raisebox{-0.5\height}{\igr{0.12}{0.cm}{0.cm}{0.cm}{0.cm}
{out_imgs/sim_comparisons/globe_ours/pred_000_normal.png}}&
\\
%%%%%%%%%%%%%%%%%%%%%%%%%%%%%%%
\rotatebox[origin=c]{90}{Truth}&
% \raisebox{-0.5\height}{\igr{0.12}{2.2cm}{2.2cm}{1.6cm}{1.6cm}
\raisebox{-0.5\height}{\igr{0.12}{0.cm}{0.cm}{0.cm}{0.cm}
{out_imgs/sim_comparisons/globe_ours/gt_000_s0.png}}&
\raisebox{-0.5\height}{\igr{0.12}{0.cm}{0.cm}{0.cm}{0.cm}
{out_imgs/sim_comparisons/globe_ours/gt_000_rgb.png}}&
\raisebox{-0.5\height}{\igr{0.12}{0.cm}{0.cm}{0.cm}{0.cm}
{out_imgs/sim_comparisons/globe_ours/gt_000_specular.png}}&
\raisebox{-0.5\height}{\igr{0.12}{0.cm}{0.cm}{0.cm}{0.cm}
{out_imgs/sim_comparisons/globe_ours/gt_000_normal.png}}&
% \\
%%%%%%%%%%%%%%%%%%%%%%%%%%%%%%%
\end{tabular}
\caption{\textbf{Comparison of reflectance separation and surface normals for polarized vs unpolarized inverse rendering}: We see that with polarimetric cues we are able to better estimate the surface normals while achieving similar reflectance separation.}
\label{fig:suppl_pol_vs_nopol}
\end{figure}
